# Supplementary material for: Orbital Energies Are Chemical Potentials in Ground-State Density Functional Theory and Excited-State $\Delta$SCF Theory
Source: arXiv:2408.10059 ancillary file (2024-08-19)
Supplement: Supplementary file 1 [file ExcitedStateChemicalPotential_SI.pdf]

# Supplemental Material: Orbital Energies Are Chemical Potentials in Ground-State Density Functional Theory and Excited-State ΔSCF Theory

Weitao Yang

*Department of Chemistry and Department of Physics, Duke University, Durham, North Carolina 27708*[*]

Yichen Fan

*Department of Chemistry, Duke University, Durham, North Carolina 27708*

**CONTENTS**

I. Orbital energies and chemical potentials in excited state OEP 2

II. Computational Details 3

A. Excited State to Excited State Chemical Potentials from Orbital Energies 3

1. OH radical and its (N±1)-systems 4

2. CO molecule and its (N±1)-systems 5

3. F atom and its (N-1)-systems 6

B. Excited State to Ground State Chemical Potentials from Orbital Energies 6

References 10

## I. ORBITAL ENERGIES AND CHEMICAL POTENTIALS IN EXCITED STATE OEP

In the excited-state optimized effective potential (OEP) approach, instead of using $\gamma_s(\mathbf{x},\mathbf{x}')$ as the basic variable, it is more convenient to use the equivalent variables $\{n_s, v_s(\mathbf{x})\}$[1]. The total excited state energy is $E_v^{n_s}(OEP) = E_v\left[n_s, v_s(\mathbf{x})\right]$ when $\frac{\delta E_v[n_s,v_s(\mathbf{x})]}{\delta v_s(\mathbf{x})} = 0$. The excited-state chemical potential expression can be derived, following the approach for ground state OEP [2]

$$
\begin{aligned}
\frac{\partial E_v\left[n_s, v_s(\mathbf{x})\right]}{\partial f_q} &= \int d\mathbf{x} \frac{\delta E_v\left[n_s, v_s(\mathbf{x})\right]}{\delta v_s(\mathbf{x})}\frac{\partial v_s(\mathbf{x})}{\partial f_q} + \left(\frac{\partial E_v\left[n_s, v_s(\mathbf{x})\right]}{\partial f_q}\right)_{v_s} \\
&= \left(\frac{\partial E_v\left[n_s, v_s(\mathbf{x})\right]}{\partial f_q}\right)_{\{\phi_p^{OEP}\}} \\
&= \left\langle \phi_p^{OEP} \left| h_{\text{eff}} \right| \phi_p^{OEP} \right\rangle \\
&= \left\langle \phi_p^{OEP} \left| h_s^{OEP} + h_{\text{eff}} - h_s^{OEP} \right| \phi_p^{OEP} \right\rangle \\
&= \varepsilon_q^{OEP} + \left\langle \phi_p^{OEP} \left| h_{\text{eff}} - h_s^{OEP} \right| \phi_p^{OEP} \right\rangle \\
&= \varepsilon_q^{OEP} + \left\langle \phi_p^{OEP} \left| v_{\text{eff}}(\mathbf{x},\mathbf{x}') - v_s(\mathbf{x})\delta(\mathbf{x},\mathbf{x}') \right| \phi_p^{OEP} \right\rangle
\end{aligned}
$$

where we used the OEP orbital equations $h_s^{OEP}\left|\phi_q^{OEP}\right\rangle = \varepsilon_q^{OEP}\left|\phi_q^{OEP}\right\rangle$ with a local potential in the Hamiltonian $h_s^{OEP} = t + v_{\text{s}}(\mathbf{x})$ . Therefore, the chemical potential is not equal to

* weitao.yang@duke.edu

OEP orbital energy in general.

## II. COMPUTATIONAL DETAILS

### A. Excited State to Excited State Chemical Potentials from Orbital Energies

Tables I-III display the excited-state chemical potentials for the OH, CO, and F atoms, including their $N \pm 1$-systems. These values are derived from the orbital energies obtained using density functional approximations (DFA) and lrLOSC-DFAs[3–7], along with calculations of $\Delta$ -SCF and the equation of motion coupled cluster single and double (EOM-CCSD). All DFT calculations were performed with QM$^4$D [8], and the EOM-CCSD calculations were performed with pySCF[9]. Valence triple-zeta polarization with diffuse functions (Def2-TZVPD)[10] basis set was utilized for all calculations. Figure 1 in the main text is based on the data provided in Table I.

### 1. *OH radical and its (N±1)-systems*

| Molecular Orbital | Chemical Potential | $\varepsilon_{\text{BLYP}}$ | $\varepsilon_{\text{lrLOSC-BLYP}}$ | Δ-BLYP | EOM-CCSD |
|---|---|---|---|---|---|
| $(\sigma_\alpha^*)^0$ | $\mu^+_{^3\Pi,^4\Pi}$(N=8) | 9.619 | 7.025 | 5.936 | 6.245 |
| $(\sigma_\alpha^*)^1$ | $\mu^-_{^4\Pi,^3\Pi}$(N=9) | 2.233 | 5.495 | | |
| $(2p_{x,\beta})^0$ | $\mu^+_{^3\Sigma^-,^2\Pi}$(N=8) | 19.346 | 13.385 | 13.279 | 12.842 |
| $(2p_{x,\beta})^1$ | $\mu^-_{^2\Pi,^3\Sigma^-}$(N=9) | 7.350 | 12.985 | | |
| $(\sigma_\beta)^0$ | $\mu^+_{^3\Pi,^2\Pi}$(N=8) | 22.754 | 17.211 | 16.876 | 16.652 |
| $(\sigma_\beta)^1$ | $\mu^-_{^2\Pi,^3\Pi}$(N=9) | 11.005 | 16.709 | | |
| $(\sigma_\beta)^0$ | $\mu^+_{^4\Pi,^3\Pi}$(N=9) | 13.828 | 9.744 | 9.400 | 8.716 |
| $(\sigma_\beta)^1$ | $\mu^-_{^3\Pi,^4\Pi}$(N=10) | 4.786 | 9.498 | | |
| $(\sigma_\beta^*)^0$ | $\mu^+_{^2\Pi,^3\Pi}$(N=9) | 0.518 | -2.060 | -1.549 | -1.691 |
| $(\sigma_\beta^*)^1$ | $\mu^-_{^3\Pi,^2\Pi}$(N=10) | -3.861 | -2.026 | | |
| $(2p_{y,\beta})^0$ | $\mu^+_{^2\Pi,^1\Sigma^+}$(N=9) | 6.527 | 1.709 | 1.965 | 1.519 |
| $(2p_{y,\beta})^1$ | $\mu^-_{^1\Sigma^+,^2\Pi}$(N=10) | -2.127 | 1.348 | | |

TABLE I. Excited state chemical potentials calculated from orbital energies for hydroxyl radical (OH) in electron volts (eV). The first column shows the relevant molecular orbital with its occupation number in super script. The chemical potentials are expressed with molecular term symbols to label the excited states involved, with the number of electrons in parenthesis to indicate the particle number in the ΔSCF calculation. The table includes chemical potentials between the ground state ($^2\Pi$) and the excited states ($^4\Pi$) of OH and the ground state ($^3\Sigma^-$) and the excited state ($^3\Pi$) of $OH^+$, as well as the chemical potentials between the the ground state ($^2\Pi$) and the excited states ($^4\Pi$) of OH and the ground state ($1\Sigma^+$) and the excited state ($^3\Pi$) of $OH^-$.

### *2. CO molecule and its (N±1)-systems*

| Molecular Orbital | Chemical Potential | $\varepsilon_{\text{B3LYP}}$ | $\varepsilon_{\text{lrLOSC-B3LYP}}$ | Δ-B3LYP | EOM-CCSD |
|---|---|---|---|---|---|
| $(\sigma^*_\beta)^0$ | $\mu^{+}_{^2\Pi,^1\Pi}$(N=13) | 10.493 | 6.473 | 6.800 | 6.855 |
| $(\sigma^*_\beta)^1$ | $\mu^{-}_{^1\Pi,^2\Pi}$(N=14) | 3.224 | 6.628 | | |
| $(\sigma^*_\alpha)^0$ | $\mu^{+}_{^2\Pi,^3\Pi}$(N=13) | 12.351 | 8.529 | 8.520 | 8.656 |
| $(\sigma^*_\alpha)^1$ | $\mu^{-}_{^3\Pi,^2\Pi}$(N=14) | 4.764 | 8.388 | | |
| $(\sigma^*_\beta)^0$ | $\mu^{+}_{^2\Sigma^+,^1\Sigma^+}$(N=13) | 17.682 | 15.363 | 14.190 | 14.165 |
| $(\sigma^*_\beta)^1$ | $\mu^{-}_{^1\Sigma^+,^2\Sigma^+}$(N=14) | 10.530 | 14.188 | | |
| $(\pi_\beta)^0$ | $\mu^{+}_{^2\Pi,^1\Sigma^+}$(N=13) | 21.131 | 17.049 | 17.105 | 17.039 |
| $(\pi_\beta)^1$ | $\mu^{-}_{^1\Sigma^+,^2\Pi}$(N=14) | 13.171 | 16.974 | | |

TABLE II. Excited state chemical potentials calculated from orbital energies for carbon monoxide (CO) in eV. The first column shows the relevant molecular orbital with its occupation number in super script. The chemical potentials are expressed with molecular term symbols to label the excited states involved, with the number of electrons in parenthesis to indicate the particle number in the ΔSCF calculation. The table includes chemical potentials between the ground state ($^1\Sigma^+$) and the excited states ($^1\Pi,^3\Pi$) of CO and the ground state ($^2\Sigma^+$) and the excited state ($^2\Pi$) of $CO^+$. The spin purification [11, 12] has been applied to $\mu^{+}_{^2\Pi,^1\Pi}$ and $\mu^{-}_{^1\Pi,^2\Pi}$ in Δ-B3LYP[13–15] and orbital energy calculations.

*3. F atom and its (N-1)-systems*

| Molecular Orbital | Chemical Potential | $\varepsilon_{\text{PBE}}$ | $\varepsilon_{\text{lrLOSC-PBE}}$ | Δ-PBE | EOM-CCSD |
|---|---|---|---|---|---|
| $(2p_{z,\beta})^0$ | $\mu^{+}_{^5S,^4P}$(N=8) | 34.608 | 27.315 | 26.687 | 27.481 |
| $(2p_{z,\beta})^1$ | $\mu^{-}_{^4P,^5S}$(N=9) | 18.597 | 26.604 | | |

TABLE III. Excited state chemical potentials calculated from orbital energies for F atom in eV. The first column shows the relevant atomic orbital with its occupation number in super script. The chemical potentials are expressed with atomic term symbols to label the excited states involved, with the number of electrons in parenthesis to indicate the particle number in the ΔSCF calculation. The table includes chemical potentials between the excited states ($^4P$) of F and the excited state ($^5S$) of $F^+$.

## B. Excited State to Ground State Chemical Potentials from Orbital Energies

Table IV displays the statistical results of 66 excited state chemical potentials derived from BLYP[13, 14] and lrLOSC-BLYP orbital energies. Reference values from experiments and IP-EOM-CCSD, along with molecular geometries, are sourced from Ranasinghe's[16] benchmark study on vertical ionization potentials, and in this study only small molecules (less than 5 atoms) were tested. All computations utilized the correlation-consistent polarized valence triple-zeta (cc-pVTZ)[17] basis set. Detailed raw data related to this test set can be found in Table V.

| | BLYP | lrLOSC-BLYP | BLYP | lrLOSC-BLYP | ΔBLYP |
|---|---|---|---|---|---|
| | $\mu^{-}_{0,n}$(N) | $\mu^{-}_{0,n}$(N) | $\mu^{+}_{n,0}$(N-1) | $\mu^{+}_{n,0}$(N-1) | |
| Highest Occupied Molecular Orbital (22 states) | | | | | |
| MAE Vs. experiment | 4.89 | 0.25 | 4.38 | 0.36 | 0.26 |
| MAE Vs. IP-EOM-CCSD | 4.85 | 0.24 | 4.44 | 0.35 | 0.26 |
| Lower occupied states (44 states) | | | | | |
| MAE Vs. experiment | 4.93 | 0.32 | 4.70 | 0.38 | 0.34 |
| MAE Vs. IP-EOM-CCSD | 5.13 | 0.32 | 4.50 | 0.40 | 0.39 |
| All valence states (66 states) | | | | | |
| MAE Vs. experiment | 4.92 | 0.30 | 4.59 | 0.37 | 0.31 |
| MAE Vs. IP-EOM-CCSD | 5.04 | 0.29 | 4.48 | 0.38 | 0.35 |

TABLE IV. Excited-state chemical potentials from HOMO and other valence states. All computations utilized the cc-pVTZ basis set, with error values reported in eV. The symmetry in chemical potentials, $\mu^{+}_{mn}(N-1) = \mu^{-}_{nm}(N)$, was preserved not only for HOMO but also for other valence states using lrLOSC.

| Molecule | Symmetry | Experiment | EOM-CCSD | Singles % | BLYP $\mu^{-}_{0,ex}(N)$ | lrLOSC $\mu^{-}_{0,ex}(N)$ | BLYP $\mu^{+}_{ex,0}(N-1)$ | lrLOSC $\mu^{+}_{ex,0}(N-1)$ | ΔBLYP |
|---|---|---|---|---|---|---|---|---|---|
| **HCN** | $1\pi$ | 13.61 | 13.89 | *95.56* | 8.81 | 13.55 | 18.47 | 13.59 | 13.61 |
| **C2H2** | $1\pi_u$ | 11.49 | 11.54 | *95.82* | 6.96 | 11.21 | 15.59 | 11.25 | 11.26 |
| **C2H2** | $3\sigma_g$ | 16.70 | 17.25 | *92.80* | 12.14 | 17.22 | 21.12 | 16.82 | 16.61 |
| **C2H2** | $2\sigma_u$ | 18.70 | 19.15 | *89.69* | 13.95 | 19.02 | | | |
| **C2H2** | $2\sigma_g$ | 23.50 | 24.43 | *79.38* | 18.36 | 23.39 | 29.02 | 23.51 | 23.59 |
| **HCCF** | $2\pi$ | 11.50 | 11.49 | *95.69* | 6.80 | 11.00 | 15.26 | 11.00 | 11.02 |
| **HCCF** | $1\pi$ | 18.00 | 18.12 | *91.37* | 12.47 | 17.72 | 23.53 | 17.90 | 17.92 |
| **NNO** | $2\pi$ | 12.89 | 12.83 | *94.11* | 8.18 | 12.74 | 17.35 | 12.75 | 12.75 |
| **NNO** | $7\sigma$ | 16.38 | 16.64 | *90.24* | 11.30 | 16.26 | 20.59 | 16.73 | 16.06 |
| **NNO** | $1\pi$ | 18.23 | 19.00 | *87.85* | 13.73 | 18.53 | 23.35 | 18.54 | 18.54 |
| **C2N2** | $1\pi_g$ | 13.51 | 13.71 | *94.29* | 9.12 | 13.35 | 16.69 | 13.05 | 12.89 |
| **C2N2** | $5\sigma_g$ | 14.49 | 14.66 | *89.97* | 9.94 | 14.44 | 17.48 | 13.79 | 13.71 |
| **C2N2** | $4\sigma_u$ | 14.86 | 15.04 | *89.50* | 10.25 | 14.75 | 17.77 | 13.93 | 14.01 |
| **CO** | $5\sigma$ | 14.01 | 14.14 | *93.23* | 8.93 | 13.94 | 18.60 | 15.12 | 13.87 |
| **CO** | $1\pi$ | 16.91 | 17.01 | *93.61* | 11.62 | 17.01 | 22.60 | 17.09 | 17.09 |
| **CO** | $4\sigma$ | 19.72 | 19.74 | *90.42* | 13.93 | 19.61 | 25.35 | 19.99 | 19.66 |
| **CO2** | $1\pi_g$ | 13.79 | 13.70 | *93.39* | 8.87 | 13.50 | 18.17 | 13.51 | 13.51 |
| **CO2** | $1\pi_u$ | 17.60 | 17.95 | *90.47* | 12.49 | 17.92 | 22.08 | 17.44 | 17.27 |
| **CO2** | $1\pi_u$ | 17.60 | 17.95 | *90.47* | 12.52 | 17.24 | 22.07 | 17.23 | 17.27 |
| **OCS** | $2\pi$ | 11.24 | 11.20 | *94.47* | 7.26 | 11.08 | 14.87 | 11.06 | 11.06 |
| **OCS** | $1\pi$ | 15.53 | 16.14 | *91.71* | 11.47 | 15.74 | 19.44 | 15.42 | 15.45 |
| **OCS** | $1\pi$ | 15.53 | 16.14 | *91.71* | 11.55 | 15.70 | 19.72 | 15.67 | 15.65 |
| **FCN** | $2\pi$ | 13.65 | 13.70 | *95.29* | 8.52 | 13.16 | 17.85 | 13.16 | 13.18 |
| **FCN** | $7\sigma$ | 14.56 | 14.44 | *91.64* | 9.36 | 14.30 | 18.84 | 15.23 | 14.25 |
| **FCN** | $1\pi$ | 19.30 | 19.67 | *91.92* | 13.70 | 19.16 | 25.09 | 19.34 | 19.33 |
| **N2** | $3\sigma_g$ | 15.58 | 15.57 | *93.14* | 10.13 | 15.26 | 20.60 | 15.30 | 15.33 |
| **N2** | $1\pi_u$ | 16.93 | 17.17 | *96.00* | 11.38 | 16.77 | 22.36 | 16.82 | 16.84 |
| **N2** | $2\sigma_u$ | 18.75 | 18.83 | *89.30* | 13.29 | 18.46 | 23.87 | 18.47 | 18.54 |
| **HCl** | $2\pi$ | 12.77 | 12.63 | *95.44* | 7.81 | 12.56 | 17.41 | 12.64 | 12.60 |
| **HCl** | $5\sigma$ | 16.60 | 16.64 | *95.12* | 11.57 | 16.45 | 21.26 | 16.56 | 16.43 |
| **HCl** | $4\sigma$ | 25.80 | 25.69 | *63.22* | 20.89 | 26.19 | 31.89 | 26.18 | 26.31 |
| **HF** | $1\pi$ | 16.19 | 15.82 | *94.84* | 9.13 | 16.01 | 23.11 | 16.29 | 16.13 |
| **HF** | $3\sigma$ | 19.90 | 19.75 | *95.60* | 12.98 | 19.75 | 26.60 | 20.07 | 19.82 |
| **F2** | $1\pi_g$ | 15.87 | 15.51 | *92.87* | 9.21 | 15.18 | 21.39 | 15.21 | 15.26 |
| **F2** | $1\pi_u$ | 18.80 | 18.82 | *90.45* | 12.56 | 18.45 | 24.59 | 18.46 | 18.54 |
| **F2** | $3\sigma_g$ | 21.10 | 21.05 | *95.47* | 15.04 | 21.05 | 27.07 | 21.12 | 21.06 |
| **SiO** | $7\sigma$ | 11.61 | 11.43 | *94.20* | 7.27 | 11.10 | 15.12 | 11.13 | 11.17 |
| **SiO** | $2\pi$ | 12.19 | 11.92 | *91.76* | 7.81 | 11.87 | 16.37 | 11.95 | 12.02 |
| **SiO** | $6\sigma$ | 14.80 | 15.05 | *89.58* | 10.51 | 14.55 | 18.94 | 14.48 | 14.66 |
| **CS** | $7\sigma$ | 11.34 | 11.47 | *90.16* | 7.27 | 11.34 | 15.07 | 11.95 | 11.25 |
| **CS** | $2\pi$ | 12.90 | 12.96 | *95.20* | 8.67 | 12.78 | 16.98 | 12.79 | 12.81 |
| **CS** | $6\sigma$ | 18.03 | 17.17 | *79.98* | 12.83 | 17.16 | 21.61 | 17.14 | 17.19 |

| Molecule | Symmetry | Experiment | EOM-CCSD | Singlet % | BLYP $\mu^{-}_{0,ex}(N)$ | lrLOSC $\mu^{-}_{0,ex}(N)$ | BLYP $\mu^{+}_{ex,0}(N-1)$ | lrLOSC $\mu^{+}_{ex,0}(N-1)$ | ΔBLYP |
|---|---|---|---|---|---|---|---|---|---|
| **P2** | $2\pi_u$ | 10.65 | 10.56 | *95.61* | 6.85 | 10.26 | 13.76 | 10.29 | 10.29 |
| **P2** | $5\sigma_g$ | 10.84 | 10.74 | *93.88* | 7.01 | 10.42 | 13.98 | 10.31 | 10.48 |
| **H2CO** | $2b_2$ | 10.90 | 10.76 | *93.57* | 6.08 | 10.64 | 15.26 | 10.63 | 10.65 |
| **H2CO** | $1b_1$ | 14.50 | 14.55 | *93.53* | 9.82 | 14.56 | 19.42 | 14.58 | 14.60 |
| **H2CO** | $5a_1$ | 16.10 | 16.03 | *92.48* | 10.77 | 15.81 | 20.61 | 15.78 | 15.71 |
| **H2CO** | $1b_2$ | 17.00 | 17.44 | *91.51* | 12.06 | 16.74 | 21.55 | 16.76 | 16.78 |
| **H2CO** | $4a_1$ | 21.40 | 21.72 | *89.12* | 15.60 | 20.51 | 25.49 | 20.57 | 20.53 |
| **H2O** | $1b_1$ | 12.62 | 12.40 | *94.45* | 6.76 | 12.56 | 18.41 | 12.76 | 12.60 |
| **H2O** | $3a_1$ | 14.74 | 14.63 | *94.69* | 8.86 | 14.69 | 20.50 | 15.05 | 14.71 |
| **H2O** | $1b_2$ | 18.55 | 18.81 | *95.67* | 12.79 | 18.66 | 24.63 | 18.82 | 18.71 |
| **H2CS** | $1b_{3u}$ | 9.38 | 9.27 | *94.34* | 5.34 | 9.17 | 12.94 | 9.17 | 9.14 |
| **H2CS** | $1b_{3g}$ | 11.76 | 11.84 | *95.23* | 7.86 | 11.68 | 15.56 | 11.68 | 11.69 |
| **H2CS** | $3a_g$ | 13.85 | 13.99 | *93.24* | 9.60 | 13.62 | 17.62 | 13.60 | 13.60 |
| **H2CS** | $1b_{2u}$ | 15.20 | 15.98 | *87.66* | 11.32 | 15.46 | 19.51 | 15.51 | 15.43 |
| **H2CS** | $2b_{1u}$ | 19.90 | 19.50 | *77.92* | 14.80 | 18.88 | 23.03 | 18.85 | 18.90 |
| **NSF** | $13a'$ | 11.82 | 11.76 | *93.17* | 7.40 | 11.47 | 15.52 | 11.46 | 11.46 |
| **NSF** | $12a'$ | 13.50 | 13.52 | *92.07* | 8.82 | 13.21 | 16.94 | 12.98 | 12.87 |
| **NSF** | $3a''$ | 13.87 | 13.92 | *94.03* | 9.22 | 13.33 | 17.47 | 13.31 | 13.33 |
| **O3** | $6a_1$ | 12.73 | 12.74 | *92.07* | 7.71 | 12.60 | 17.25 | 12.26 | 12.46 |
| **O3** | $4b_2$ | 13.00 | 12.87 | *91.60* | 7.84 | 12.73 | 17.54 | 12.61 | 12.68 |
| **O3** | $1a_2$ | 13.54 | 13.43 | *92.88* | 8.88 | 13.57 | 18.14 | 13.59 | 13.53 |
| **O3** | $1b_1$ | 16.50 | 18.80 | *67.42* | 14.22 | 19.10 | 24.06 | 19.10 | 19.13 |
| **NH3** | $3a_1$ | 10.80 | 10.73 | *94.42* | 5.79 | 10.82 | 15.74 | 11.25 | 10.82 |
| **NH3** | $1\varepsilon$ | 16.00 | 16.48 | *95.23* | 11.04 | 16.23 | 21.41 | 16.39 | 16.24 |
| MAE exp | | | | | 4.92 | 0.30 | 4.59 | 0.37 | 0.31 |
| MAE EOM-CCSD | | | | | 5.04 | 0.29 | 4.48 | 0.38 | 0.35 |

TABLE V. Excited-state chemical potentials from HOMO and other valence states in unit of eV. BLYP broke the π symmetry in CO2 and OCS molecules and chemical potentials from both symmetry-breaking states were reported in red.

[1] W. Yang and P. W. Ayers, Foundation for the ΔSCF Approach in Density Functional Theory (2024), arXiv:2403.04604.

[2] A. J. Cohen, P. Mori-Sánchez, and W. Yang, Fractional charge perspective on the band gap in density-functional theory, Physical Review B **77**, 115123 (2008).

[3] C. Li, X. Zheng, N. Q. Su, and W. Yang, Localized orbital scaling correction for systematic elimination of delocalization error in density functional approximations, National Science Review **5**, 203 (2018).

[4] N. Q. Su, A. Mahler, and W. Yang, Preserving Symmetry and Degeneracy in the Localized Orbital Scaling Correction Approach, The Journal of Physical Chemistry Letters **11**, 1528 (2020).

[5] Y. Mei, Z. Chen, and W. Yang, Exact second-order corrections and accurate quasiparticle energy calculations in density functional theory, J. Phys. Chem. Lett. **12**, 7236 (2021).

[6] J. Yu, Y. Mei, Z. Chen, and W. Yang, Accurate Prediction of Core Level Binding Energies from Ground-State Density Functional Calculations: The Importance of Localization and Screening (2024), arXiv:2406.06345 [physics].

[7] J. Z. Williams and W. Yang, Correcting Delocalization Error in Materials with Localized Orbitals and Linear-Response Screening (2024), arXiv:2406.07351 [cond-mat, physics:physics].

[8] An in-house program for qm/mm simulations. https://qm4d.org/.

[9] Q. Sun, X. Zhang, S. Banerjee, P. Bao, M. Barbry, N. S. Blunt, N. A. Bogdanov, G. H. Booth, J. Chen, Z. H. Cui, J. J. Eriksen, Y. Gao, S. Guo, J. Hermann, M. R. Hermes, K. Koh, P. Koval, S. Lehtola, Z. Li, J. Liu, N. Mardirossian, J. D. McClain, M. Motta, B. Mussard, H. Q. Pham, A. Pulkin, W. Purwanto, P. J. Robinson, E. Ronca, E. R. Sayfutyarova, M. Scheurer, H. F. Schurkus, J. E. Smith, C. Sun, S. N. Sun, S. Upadhyay, L. K. Wagner, X. Wang, A. White, J. D. Whitfield, M. J. Williamson, S. Wouters, J. Yang, J. M. Yu, T. Zhu, T. C. Berkelbach, S. Sharma, A. Y. Sokolov, and G. K. L. Chan, Recent developments in the p y scf program package, J. Chem. Phys. **153**, 24109 (2020).

[10] R. Gulde, P. Pollak, and F. Weigend, Error-Balanced Segmented Contracted Basis Sets of Double-$\zeta$ to Quadruple-$\zeta$ Valence Quality for the Lanthanides, J. Chem. Theory Comput. **8**, 4062 (2012), publisher: American Chemical Society.

[11] T. Ziegler, A. Rauk, and E. J. Baerends, On the calculation of multiplet energies by the hartree-fock-slater method, Theoretica chimica acta **43**, 261 (1977).

[12] T. Kowalczyk, S. R. Yost, and T. V. Voorhis, Assessment of the $\delta$SCF density functional theory approach for electronic excitations in organic dyes, The Journal of Chemical Physics **134**, 054128 (2011).

[13] A. D. Becke, Density-functional exchange-energy approximation with correct asymptotic behavior, Phys. Rev. A **38**, 3098 (1988).

[14] C. Lee, W. Yang, and R. G. Parr, Development of the colle-salvetti correlation-energy formula into a functional of the electron density, Phys. Rev. B **37**, 785 (1988).

[15] P. J. Stephens, F. J. Devlin, C. F. Chabalowski, and M. J. Frisch, Ab initio calculation of vibrational absorption and circular dichroism spectra using density functional force fields, J. Phys. Chem. **98**, 11623 (1994).

[16] D. S. Ranasinghe, J. T. Margraf, A. Perera, and R. J. Bartlett, Vertical valence ionization potential benchmarks from equation-of-motion coupled cluster theory and QTP functionals, The Journal of Chemical Physics **150**, 074108 (2019).

[17] T. H. Dunning, Gaussian basis sets for use in correlated molecular calculations. I. The atoms boron through neon and hydrogen, J. Chem. Phys. **90**, 1007 (1989).
